# Supplementary material for: Optical Responses of Chiral Majorana Edge States in Two-Dimensional Topological Superconductors
Source: arXiv:2106.05246 source file (2021-06-09)
Supplement: Supplementary file 1 [file Supplementary.pdf]

# 1 Optical conductivity in eigenstate representation

The linear response conductivity is ($\hbar = 1$ is used for convenience)

$$\sigma_{ab}(\boldsymbol{r},\omega) = \frac{\Sigma_{ab}(\boldsymbol{r},\omega) - \Sigma_{ab}(\boldsymbol{r},0)}{\omega + i\eta} \tag{S.1}$$

with

$$\Sigma_{ab}(\boldsymbol{r},\omega) \equiv \frac{1}{2\pi V}\int_0^\infty dt e^{i(\omega+i\eta)t}\langle[J_a(\boldsymbol{r}), J_b(\boldsymbol{r})]\rangle \tag{S.2}$$

$$= \frac{i}{2\pi V}\sum_{mn}\frac{f(\epsilon_n) - f(\epsilon_m)}{\epsilon_n - \epsilon_m + (\omega + i\eta)}\langle n|J_a(\boldsymbol{r})|m\rangle\langle m|J_b(\boldsymbol{r})|n\rangle. \tag{S.3}$$

Or

$$\sigma_{ab}(\boldsymbol{r},\omega) = \frac{1}{2\pi i V}\sum_{mn}\frac{f(\epsilon_m) - f(\epsilon_n)}{\epsilon_m - \epsilon_n}\frac{\langle m|J_a(\boldsymbol{r})|n\rangle\langle n|J_b(\boldsymbol{r})|m\rangle}{\epsilon_m - \epsilon_n + \omega + i\eta} \tag{S.4}$$

where $|m\rangle$ are energy eigenstates and $f(\epsilon)$ is the Fermi-Dirac distribution function. $V$ is the volume (the area/length in 2D/1D case) of the system.

# 2 Optical conductivity in terms of Green's functions

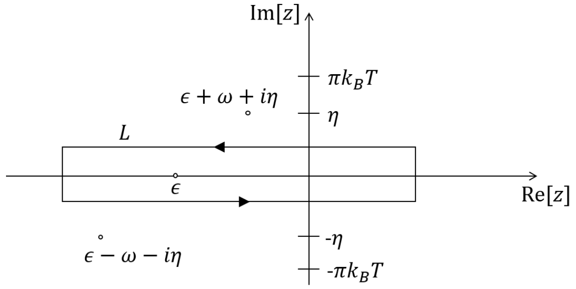


Figure 1: Contour integral.

Eq. (S.4) may be calculated using contour integral. To do that, define

$$g(z) = \frac{f(z)}{z - \epsilon_n}\frac{1}{z - \epsilon_m + \tilde{\omega}}. \tag{S.5}$$

Then we obtain

$$\oint_L g(z)dz = 2\pi i\frac{f(\epsilon_n)}{\epsilon_n - \epsilon_m + \tilde{\omega}} \tag{S.6}$$

or

$$\frac{f(\epsilon_n)}{\epsilon_n - \epsilon_m + \tilde{\omega}} = \frac{1}{2\pi i}\oint_L \frac{f(z)}{z - \epsilon_n}\frac{1}{z - \epsilon_m + \tilde{\omega}}dz. \tag{S.7}$$

Similarly, we obtain

$$\frac{-f(\epsilon_m)}{\epsilon_n - \epsilon_m + \tilde{\omega}} = \frac{1}{2\pi i}\oint_L \frac{f(z)}{z - \epsilon_m}\frac{1}{z - \epsilon_n - \tilde{\omega}}dz. \tag{S.8}$$

Substitution into Eq.(S.3) gives ( $\tilde{\omega} = \omega + i\eta$)

$$\Sigma_{ab}(\boldsymbol{r},\omega) = \frac{i}{2\pi V}\sum_{mn}\frac{1}{2\pi i}\oint_L dz[\frac{f(z)}{z-\epsilon_n}\frac{1}{z-\epsilon_m+\tilde{\omega}} + \frac{f(z)}{z-\epsilon_m}\frac{1}{z-\epsilon_n-\tilde{\omega}}]\langle n|J_a(\boldsymbol{r})|m\rangle\langle m|J_b(\boldsymbol{r})|n\rangle. \quad (S.9)$$

$$= \frac{1}{4\pi^2 V}\oint_L dz f(z)\ \mathrm{Tr}[J_a(\boldsymbol{r})G(z+\omega+i\eta)J_b(\boldsymbol{r})G(z) + J_a(\boldsymbol{r})G(z)J_b(\boldsymbol{r})G(z-\omega-i\eta)] \quad (S.10)$$

For the contour we choose,

$$\oint_L dz g(z) = \int_{-\infty}^{\infty} g(\epsilon - i\eta/2)d\epsilon - \int_{-\infty}^{\infty} g(\epsilon + i\eta/2)d\epsilon. \quad (S.11)$$

Thus, we get

$$\begin{aligned}\Sigma_{ab}(\boldsymbol{r},\omega) = {}& \frac{1}{4\pi^2 V}\int_{-\infty}^{\infty} d\epsilon f(\epsilon)\ \mathrm{Tr}[J_a(\boldsymbol{r})G(\epsilon+\omega+\frac{1}{2}i\eta)J_b(\boldsymbol{r})G(\epsilon-\frac{1}{2}i\eta) + J_a(\boldsymbol{r})G(\epsilon-\frac{1}{2}i\eta)J_b(\boldsymbol{r})G(\epsilon-\omega-\frac{3}{2}i\eta) \\ & -J_a(\boldsymbol{r})G(\epsilon+\omega+\frac{3}{2}i\eta)J_b(\boldsymbol{r})G(\epsilon+\frac{1}{2}i\eta) - J_a(\boldsymbol{r})G(\epsilon+\frac{1}{2}i\eta)J_b(\boldsymbol{r})G(\epsilon-\omega-\frac{1}{2}i\eta)] \\ = {}& \frac{1}{4\pi^2 V}\int_{-\infty}^{\infty} d\epsilon f(\epsilon)\ \mathrm{Tr}[J_a(\boldsymbol{r})G^r(\epsilon+\omega)J_b(\boldsymbol{r})G^a(\epsilon) + J_a(\boldsymbol{r})G^a(\epsilon)J_b(\boldsymbol{r})G^a(\epsilon-\omega) \\ & -J_a(\boldsymbol{r})G^r(\epsilon+\omega)J_b(\boldsymbol{r})G^r(\epsilon) - J_a(\boldsymbol{r})G^r(\epsilon)J_b(\boldsymbol{r})G^a(\epsilon-\omega)] \\ = {}& \frac{1}{4\pi^2 V}\int_{-\infty}^{\infty} d\epsilon f(\epsilon)\ \mathrm{Tr}\{J_a(\boldsymbol{r})G^r(\epsilon+\omega)J_b(\boldsymbol{r})[G^a(\epsilon)-G^r(\epsilon)] \\ & +J_b(\boldsymbol{r})G^a(\epsilon-\omega)J_a(\boldsymbol{r})[G^a(\epsilon)-G^r(\epsilon)]\}\end{aligned} \quad (S.12)$$

Particularly, the longitudinal elements are

$$\Sigma_{aa}(\boldsymbol{r},\omega) = \frac{1}{4\pi^2 V}\int_{-\infty}^{\infty} d\epsilon f(\epsilon)\ \mathrm{Tr}\{J_a(\boldsymbol{r})[G^r(\epsilon+\omega)+G^a(\epsilon-\omega)]J_a(\boldsymbol{r})[G^a(\epsilon)-G^r(\epsilon)]\}, \quad (S.13)$$

$$= \frac{1}{4\pi^2 V}\int_{-\infty}^{\infty} d\epsilon f(\epsilon)\ \mathrm{Tr}\{J_a(\boldsymbol{r})[G^r(\epsilon+\omega)+G^a(\epsilon-\omega)]J_a(\boldsymbol{r})[G^a(\epsilon)-G^r(\epsilon)]\}, \quad (S.14)$$

or

$$\Sigma_{aa}(\boldsymbol{r},\omega) = \frac{i}{\pi^2 V}\int_{-\infty}^{\infty} d\epsilon f(\epsilon)\ \mathrm{Tr}\{J_a(\boldsymbol{r})B_\omega(\epsilon)J_a(\boldsymbol{r})A_0(\epsilon)\} \quad (S.15)$$

where we defined

$$A_\omega(\epsilon) \equiv -\frac{1}{2i}[G^r(\epsilon+\omega) - G^a(\epsilon-\omega)], \quad (S.16)$$

$$B_\omega(\epsilon) \equiv \frac{1}{2}[G^r(\epsilon+\omega) + G^a(\epsilon-\omega)]. \quad (S.17)$$

Note that $\langle\epsilon_k|A_0(\epsilon)|\epsilon_k\rangle = \pi\delta(\epsilon-\epsilon_k)$ is the spectral function. Also, $\Sigma_{aa}(\boldsymbol{r},0)$ has zero real part since it is a trace of the product of a hermitian matrix and an anti-hermitian one.

$$\Re[\Sigma_{aa}(\boldsymbol{r},0)] = 0. \quad (S.18)$$

For general $\omega$,

$$\Re[\Sigma_{aa}(\boldsymbol{r},\omega)] = \frac{1}{2\pi^2 V}\int_{-\infty}^{\infty} d\epsilon f(\epsilon)\ \mathrm{Tr}\{J_a(\boldsymbol{r})[A_0(\epsilon+\omega) - A_0(\epsilon-\omega)]J_a(\boldsymbol{r})A_0(\epsilon)\}, \quad (S.19)$$

$$= \frac{1}{2\pi^2 V}\int_{-\infty}^{\infty} d\epsilon[f(\epsilon) - f(\epsilon+\omega)]\ \mathrm{Tr}\{J_a(\boldsymbol{r})A_0(\epsilon+\omega)J_a(\boldsymbol{r})A_0(\epsilon)\} \quad (S.20)$$

and thus

$$\Re[\sigma_{aa}(\boldsymbol{r},\omega)] = \frac{1}{\omega}\frac{1}{2\pi^2 V}\int_{-\infty}^{\infty} d\epsilon[f(\epsilon) - f(\epsilon+\omega)]\ \mathrm{Tr}\{J_a(\boldsymbol{r})A_0(\epsilon+\omega)J_a(\boldsymbol{r})A_0(\epsilon)\}. \quad (S.21)$$

In the case of the tight-binding model, the Greens functions $G^{r/a}(\epsilon)$ (which are matrices) can be calculated recursively, which is an advantage compared to the eigenstate method.

# 3. The derivation of Eq. (5)

The current operator $J(x)$ on the edge is not solely derived from the effective Hamiltonian in Eq. (4). It depends on the specific bulk system. The edge current operator is obtained by projecting the bulk operator onto the edge states. For example, the edge current operator in $p$-wave SCs is [*Phys. Rev. B.64.054514 (2001)*]

$$J_x^p = \sum_k \frac{e\hbar}{m} k_x \gamma_{k_x}^\dagger \gamma_{k_x}.$$

with $m$ being the bulk electron mass. This results in a local current operator

$$J_x^p(x) = \frac{e\hbar}{2mi}[\gamma\partial_x\gamma - (\partial_x\gamma)\gamma].$$

Fourier transform of this operator leads to Eq. (5) of the manuscript with $m^* = m$. In Eq. (5) $m$ is replaced by the effective mass $m^*$ for generality since it depends on the specific system.

The constant $e$ in Eq. (5) of the manuscript seems to suggest that each Majorana fermion has the same charge as an electron, contradicting the charge neutrality. To clarify that there is no real contradiction, let us consider the zero-temperature limit where there are no occupied single-particle states. The usual transition $\gamma_k^\dagger \gamma_{k'}$ cannot happen and thus the first term of Eq. (5) vanishes. The remaining terms are related to Majorana pairs $\gamma_k^\dagger \gamma_{k'}^\dagger$ (instead of single Majorana fermions) which couple with the electromagnetic field by charge $e$. Thus, Eq. (5) does not contradict the charge-neutrality of single Majorana fermions.

# 4. The temperature dependence

We have shown in the main text that the one-dimensional analysis indicates $\Re[\sigma_{xx}(T)]_{\omega=0} \sim T^2$. In Figure S1, we show the temperature dependence of $\Re[\sigma_{xx}(\omega=0)]$ in the two-dimensional $p$-wave SC model given by Eq. (1). The edge response shows a $T^2$ dependence (clearer in the inset) while the bulk response is exponentially suppressed at small $T$.

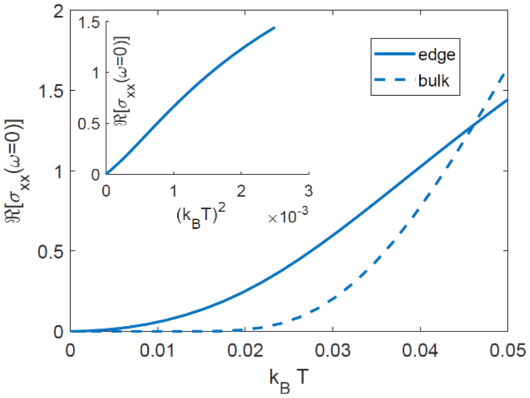


**Figure S1.** The temperature dependence of the optical conductivity. The SC gap

Note again that for normal chiral fermions, $\Re[\sigma_{xx}(\omega \ll \Delta_{gap}, T \ll \Delta_{gap})]$ is a constant independent of $\omega$ or $T$. So, the temperature dependence can also distinguish the Majorana mode signal from others.

# 5. Estimation of the measurables in realistic topological insulator-based systems

We have done a simple estimation in the manuscript, assuming the detection spot size to be about $1\mu m$ and $\Delta/\mu \sim 10^{-4}$. In this case, $\Re[\sigma_{xx}] \approx 0.1\, e^2/h$, comparable to the normal chiral fermion response $\Re^N[\sigma_{xx}] \approx 0.5\, e^2/h$. Since the latter has been detected successfully, the Majorana signal should be also detectable with a detection spot size of $1\mu m$, which is achievable experimentally. This estimation is valid for systems with $\mu$ being of the order of 1eV. A chiral $p$-wave SC (for which $Sr_2RuO_4$ may be a candidate) should belong to this category.

A recent microwave microscopy experiment has been done with a spatial resolution of $5nm$ [*Science Advances 6, eabd1919 (2020)*]. This indicates that a very small $d$ can be used to detect the Majorana modes as well. Assuming $d = 5nm$, the signal of $\Re[\sigma_{xx}]$ can reach $4000e^2/h$.

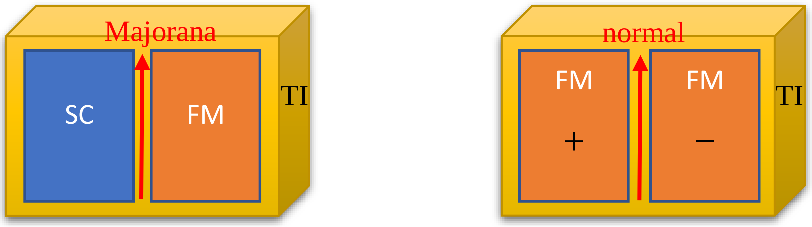


**Figure S2.** Left: chiral Majorana modes on domain boundaries of SC and ferromagnetic regions. Right: chiral normal fermions on domain walls of ferromagnets.

Realistic systems hosting chiral Majorana modes can be achieved using topological insulators (TIs) $Bi_2Se_3$ (or similar materials). One may use a thin film of $Bi_2Se_3$ in combination with magnetism and SC (such as in reference [17] of the manuscript and [*Communications Physics 2, (2019)*]). Eq. (1) of the manuscript is an effective model for such a system. One may alternatively use a bulk 3D TI instead of a thin film and introduce domains of SC and ferromagnetism (FM) [*Phys. Rev. Lett. 102, 216403(2009); Phys. Rev. Lett. 102, 216404(2009)*] as shown in the panel of Figure S2. A chiral Majorana mode appears at the SC/FM boundary. If the SC is replaced by a second FM with opposite magnetization compared to the existing one (as shown in the right panel of Figure S2), there appears a chiral normal fermion mode at the boundary. In the following, we estimate the optical conductivity of Majorana modes in such TI-based systems.

To realize Majorana modes, the chemical potential $\mu$ needs to be inside the magnetization gap $\Delta_m$. Since $\Delta_m$ can reach 50meV in magnetic TIs [*Nat. Rev. Phys. 1, 126–143(2019); Phys. Rev. B 102, 115402(2020)*], we assume $\mu = 50meV$. The superconducting gap is generated by the proximity effect and is much smaller. A reasonable estimation is $\Delta_{sc} = 0.1\ meV$. To estimate the realistic value of the detection spot size, note that a recent microwave microscopy experiment has been done with a spatial resolution of $5nm$ [*Science Advances 6, eabd1919 (2020)*]. Assuming $d = 4nm$ and $k_c = 10nm^{-1}$ in Eq. (6) of the manuscript, we estimate the peak value to be $\Re[\sigma_{xx}(\omega_0)] \approx 10\, e^2/h$ at the peak position $\hbar\omega_0/\Delta_{sc} \approx 0.03$, or $\hbar\omega_0 \approx 0.003meV$, $\omega_0 \approx 4.5$ GHz.
